# Supplementary material for: Technical Report: A Hierarchical Deliberative-Reactive System Architecture for Task and Motion Planning in Partially Known Environments
Source: arXiv:2202.01385 source file (2022-02-03)
Supplement: Supplementary file 1 [file 7-appendix.tex]

\clearpage
\section{Appendices}

\subsection{Platforms Scenario}

In this scenario, the robot must traverse a set of platforms of increasing height until reaching a goal object on the upper right.
To solve this problem, the robot must push blocks near walls to jump to the next platform, as illustrated in Fig.~\ref{fig:scenario_platforms}.
Each darker shade of grey in the figure corresponds to an increase of height from $z=0$ (white) to $z=6$, with each red block height $z=1$ relative to the plan it is one. 

This environment does not have complex walls or obstacles, so it can be solved by the planner using both the Baseline and Reactive planning approaches. 
In both cases, the addition of platforms and objects affects planning time exponentially, as platforms increase plan depth and possible objects to manipulate increase the branching factor of action selection.
However, average planning time is significantly lower when incorporating the reactive layer due to the lower number of necessary samples, as shown in Fig.~\ref{fig:results_platforms}.

\begin{figure}[h]
  \centering
    \begin{subfigure}[t]{0.2\textwidth}
      \centering
      \includegraphics[width=\textwidth]{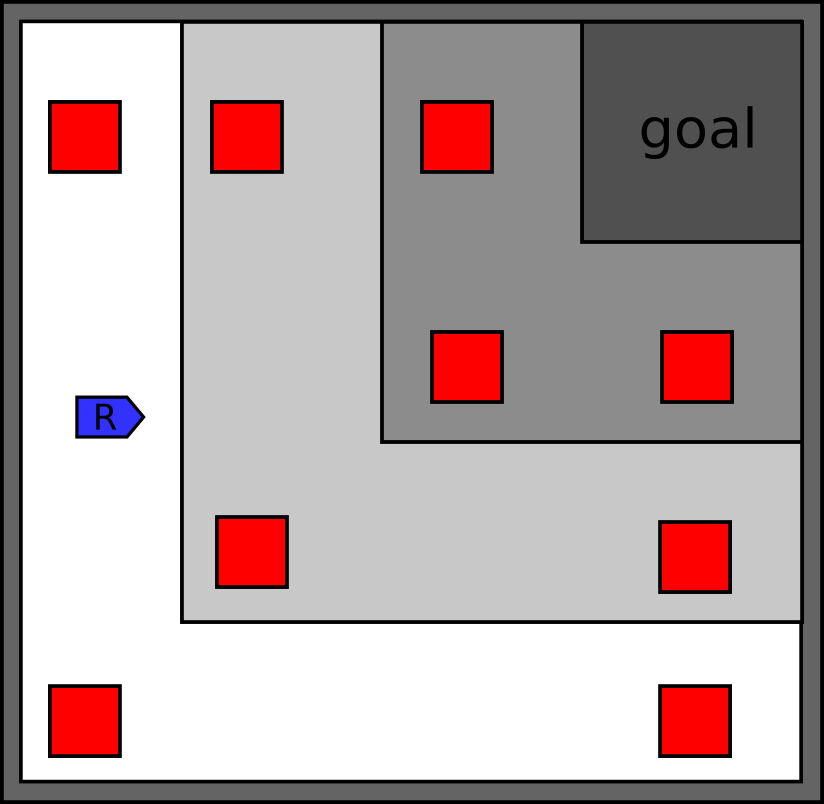}
        \caption{\small{Scenario overview}}
        \label{fig:scenario_platforms}
    \end{subfigure}
    \begin{subfigure}[t]{0.27\textwidth}
        \includegraphics[width=\textwidth]{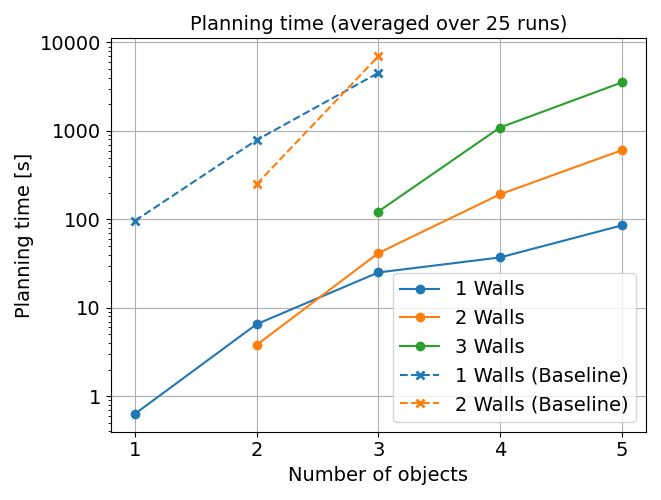}
        \caption{\small{Planning time vs. complexity}}
        \label{fig:results_platforms}
    \end{subfigure}
    \caption{%
    \textbf{Platforms scenario}. 
    The robot must push blocks to jump on platforms until reaching the goal platform on the upper right.
    Red squares denote the possible object spawn locations, which are chosen randomly so there is at least one block per level (for the task to be solvable) (a).
    Planning time increases with number of platforms and objects in both approaches. 
    However, the Baseline planning approach requires more computation due to its reliance on more samples to solve over lower-level motion primitives (b).
    \label{fig:platforms}
    }
\end{figure}

%%%%%%%%%%%%%%%%%%%
% BRIDGE SCENARIO %
%%%%%%%%%%%%%%%%%%%
\newpage

% \textcolor{red}{SC: Is this paragraph needed or should we discuss this in the conclusion as a general issue?}
% We identify some possible improvements that could increase performance in this scenario. 
% Currently, we sample poses uniformly, which can lead to challenges in fine placement tasks such as moving \texttt{B2} into the gap connecting \texttt{ramp2} and \texttt{goal}.
% Indeed, reducing the size of this gap or the robot's jump threshold distance can severely affect the success of our planner in both domains. 
% A different choice of sampling strategy, search algorithm, or search heuristic could enable solving this scenario faster and more consistently in both planning domains; however, we have chosen to solve this in our work by leveraging the reactive layer for navigation and forgoing the need to plan over fine-grained \texttt{move} actions altogether.

\begin{figure*}
\centering
\includegraphics[width=0.8\textwidth]{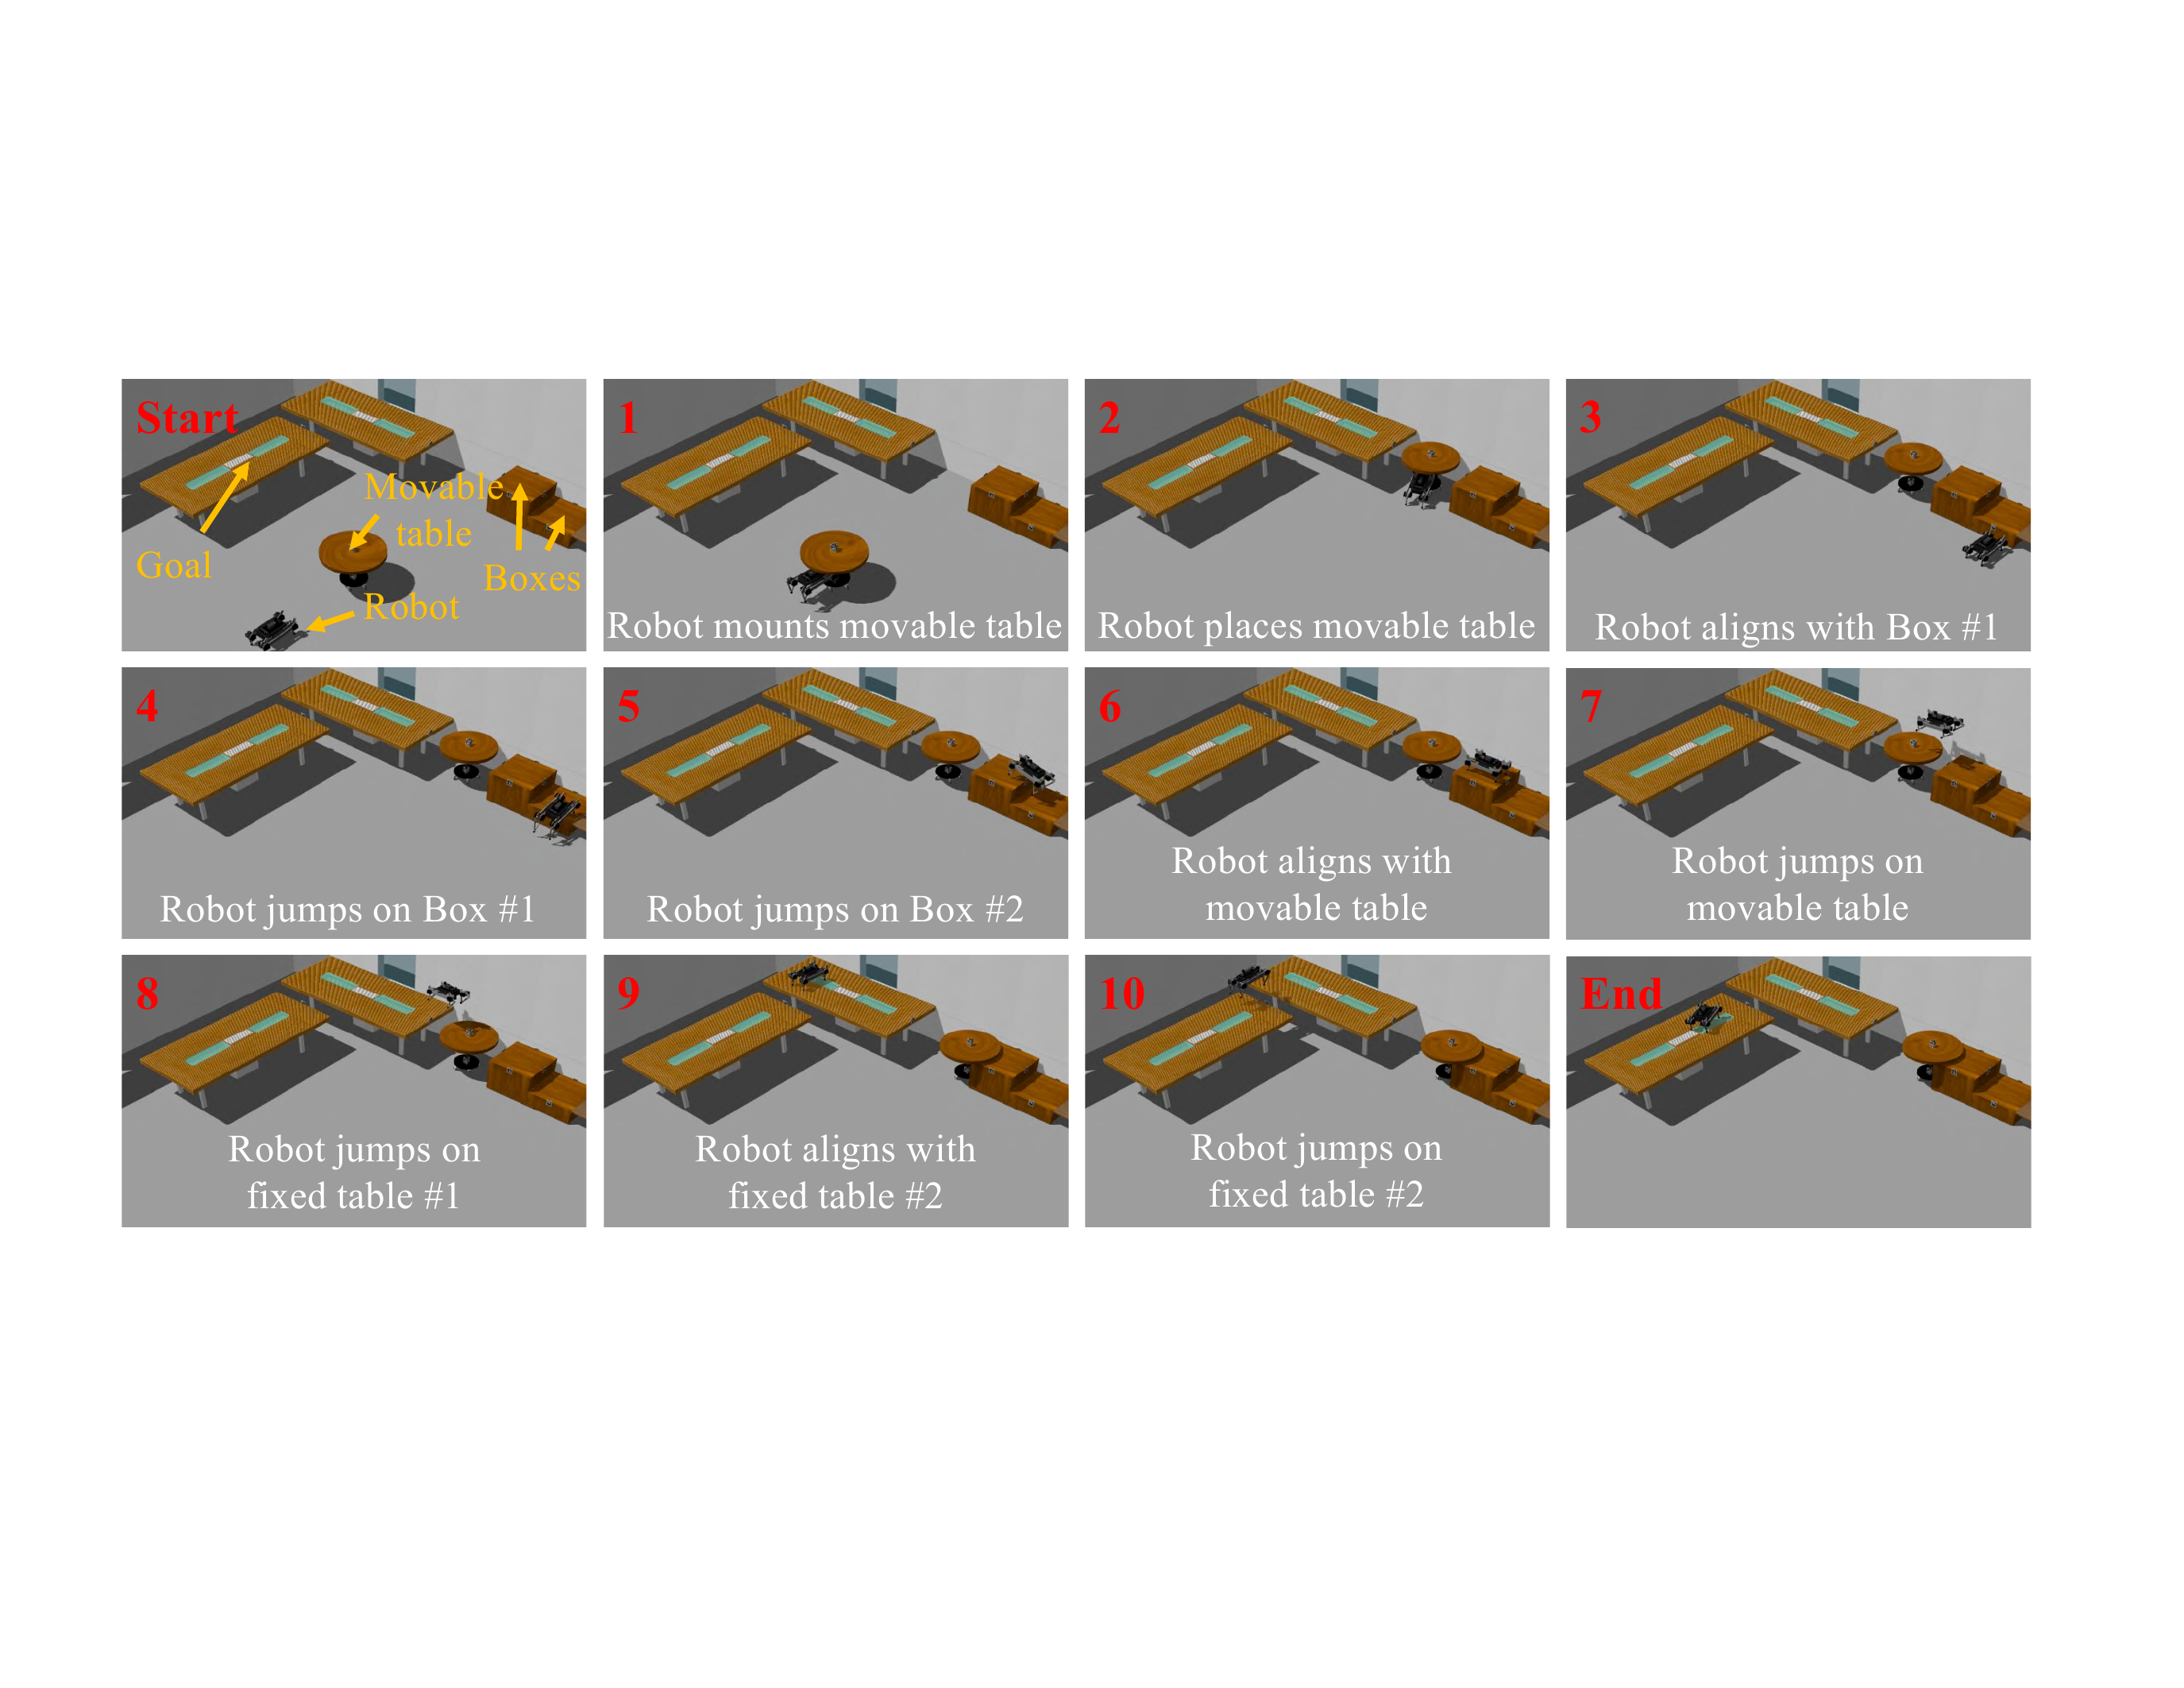}
\caption{Simulation of a variation of the \emph{Bridge} scenario using the Baseline planning approach.}
\label{fig:gazebo_bridge}
\end{figure*}

%%%%%%%%%%%%%%%%%%%%%%
% REAL-WORLD RESULTS %
%%%%%%%%%%%%%%%%%%%%%%
% \subsection{Real-World Results} 

% Fig.~\ref{fig:minitaur_experiment} shows a simple real-world scenario, in which a real Minitaur robot must clear an object obstructing its path to a goal object.
% It should be noted that we used the same software implementation of the deliberative, reactive, and gait layers in both the physical experiments and the Gazebo simulations. 

% \begin{figure*}
% \centering
% \includegraphics[width=0.825\textwidth]{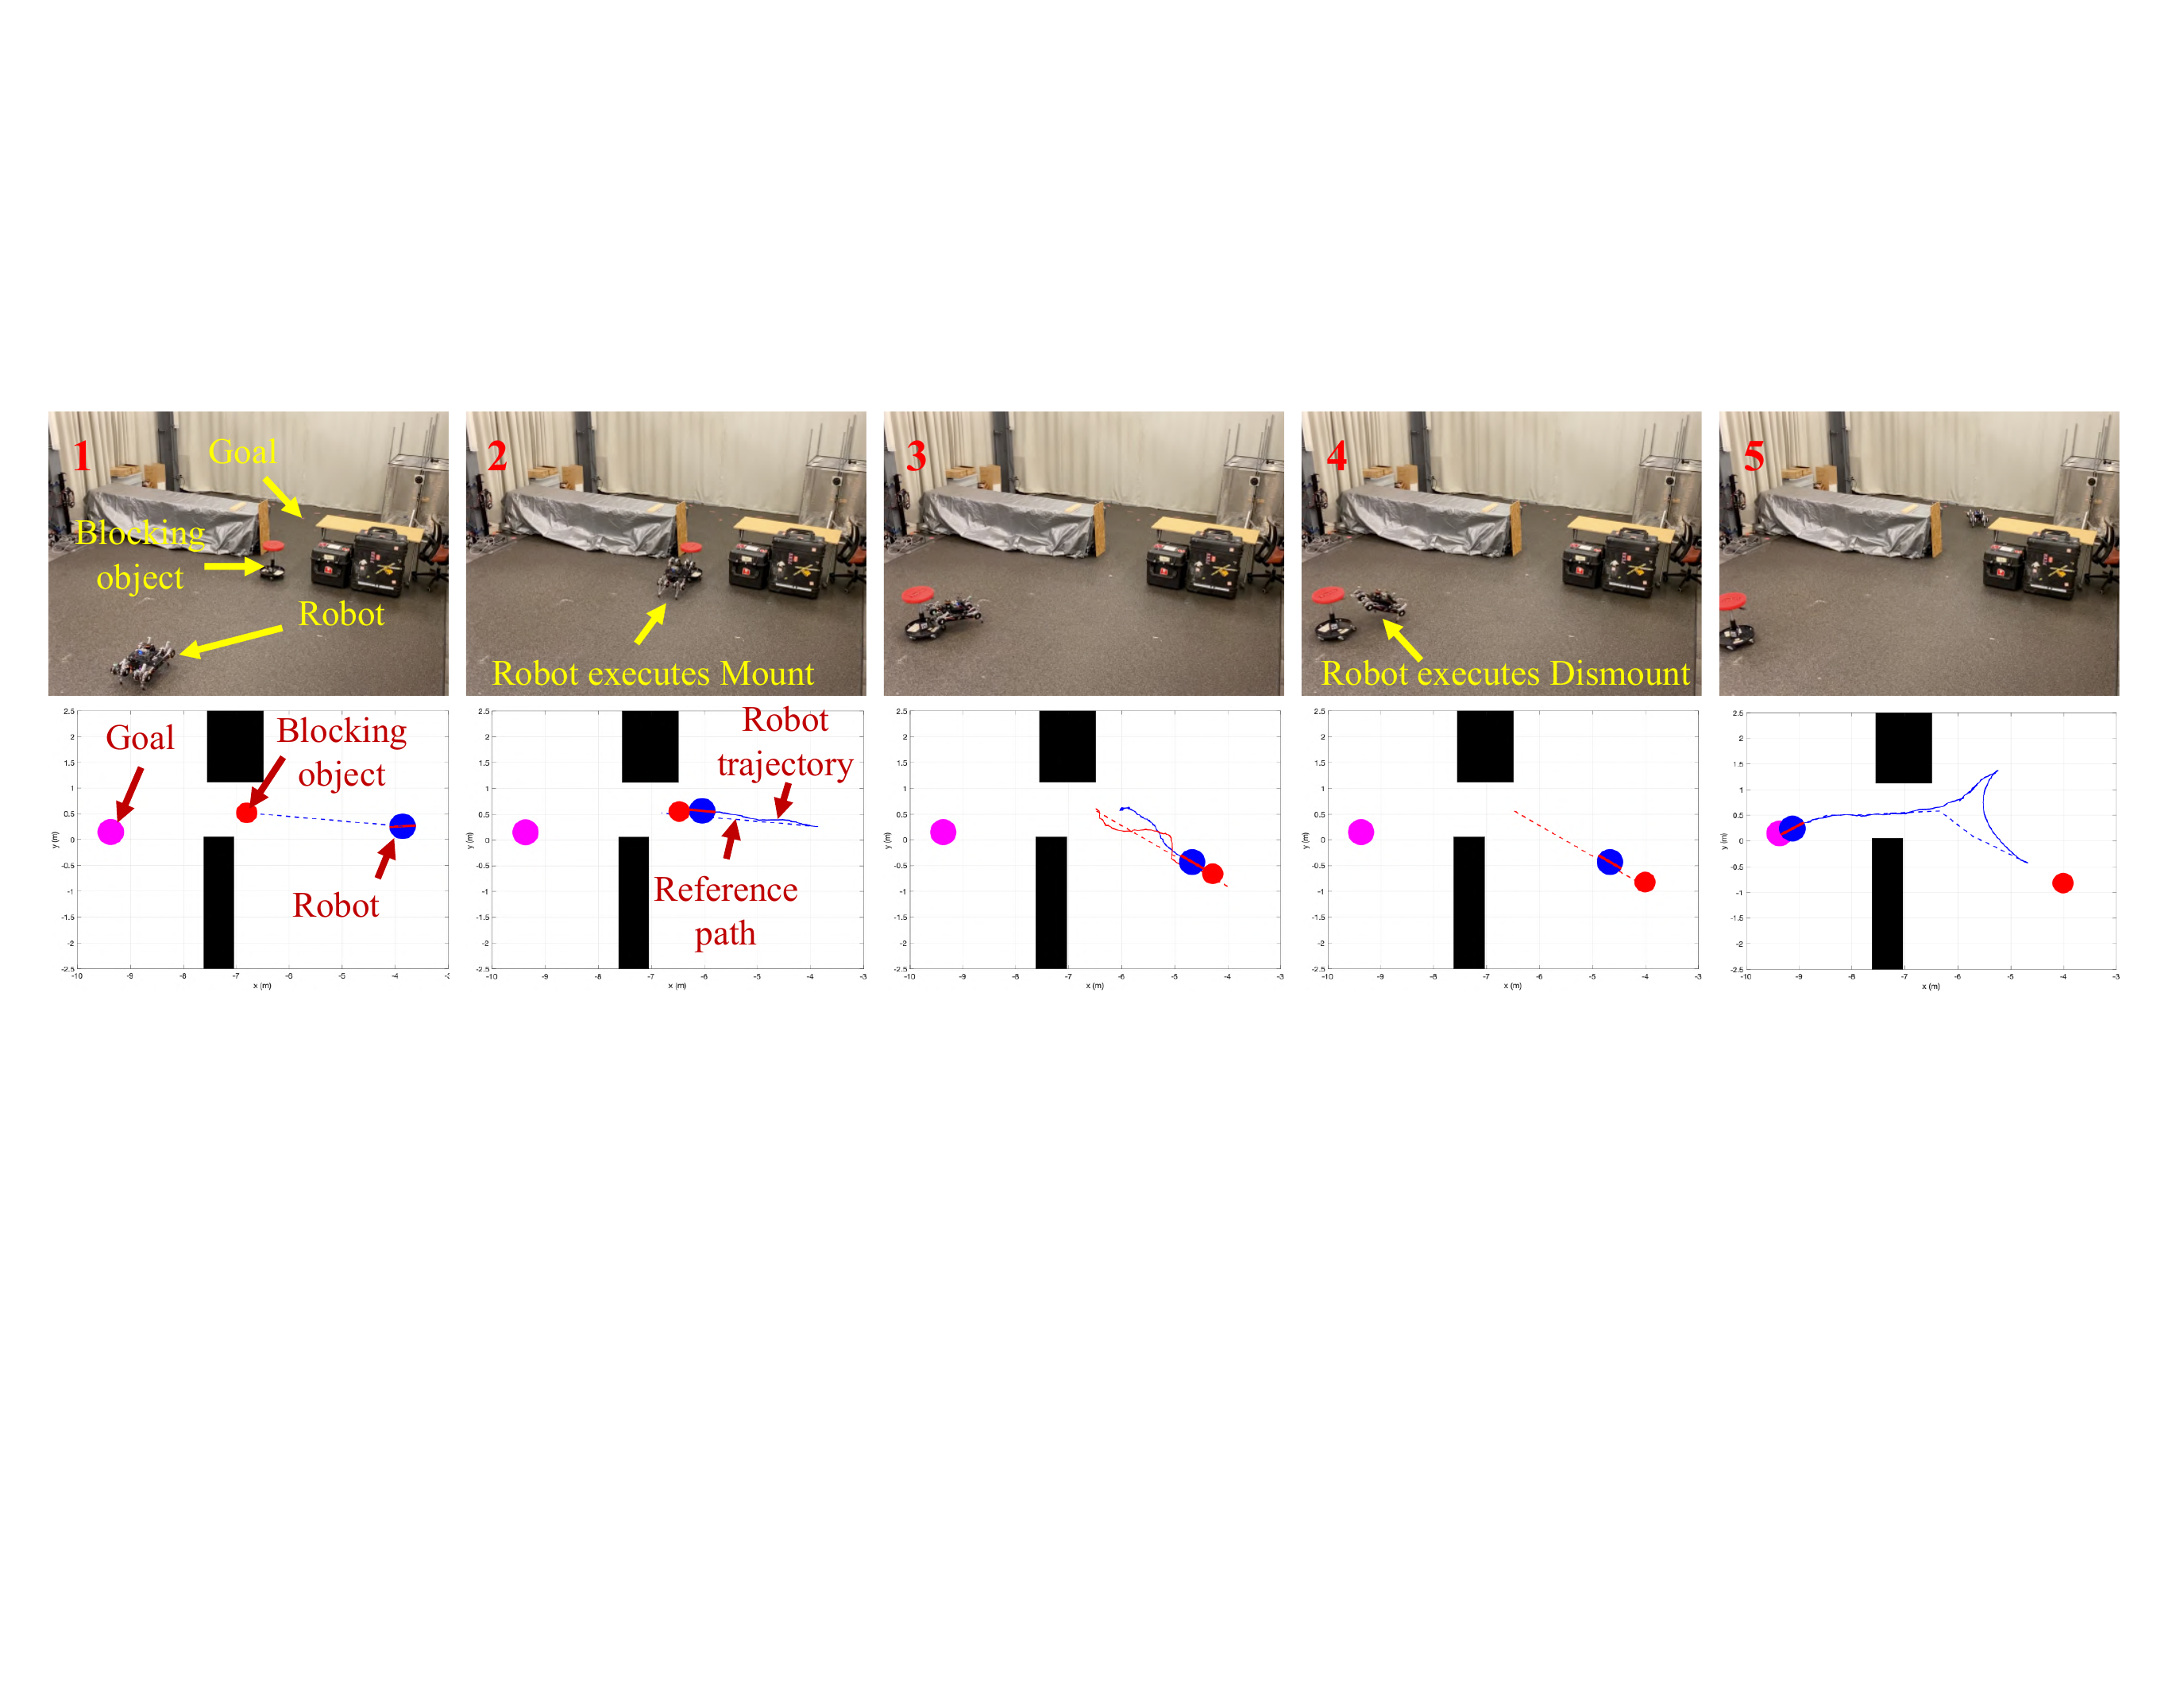}
% \caption{Real-world experiment with the Minitaur robot using the Baseline planning approach.}
% \label{fig:minitaur_experiment}
% \end{figure*}
